# Supplementary material for: Metastable and Unstable Dynamics in multi-phase lattice Boltzmann
Source: arXiv:2212.07848 ancillary file (2022-12-18)
Supplement: Supplementary file 1 [file SupplementalMaterial.pdf]

# Metastable and Unstable Dynamics in multi-phase lattice Boltzmann: Supplemental Material

Matteo Lulli,[1] Luca Biferale,[2] Giacomo Falcucci,[3] Mauro Sbragaglia,[2] Dong Yang,[1] and Xiaowen Shan[1,*]

[1]*Department of Mechanics and Aerospace Engineering, Southern University of Science and Technology, Shenzhen, Guangdong 518055, China*

[2]*Department of Physics & INFN, University of Rome "Tor Vergata", Via della Ricerca Scientifica 1, 00133 Rome, Italy.*

[3]*Department of Enterprise Engineering "Mario Lucertini", University of Rome "Tor Vergata", Via del Politecnico 1, 00133 Rome, Italy; John A. Paulson School of Engineering and Applied Physics, Harvard University, 33 Oxford Street, 02138 Cambridge, Massachusetts, USA.*

(Dated: December 15, 2022)

## I. SHAN-CHEN LATTICE BOLTZMANN MODEL

In this Section we review the fundamental aspects of the lattice Boltzmann model (LBM) in its usual notation and provide a link to the rescaled notation used in the main text. The LBM equation for a system with a local force and stochastic fluctuations can be written as [1, 2]

$$f_i(\mathbf{x}+\xi_i,t+1)-f_i(\mathbf{x},t)=\Omega_i^{(\mathrm{BGK})}(\mathbf{x},t)+F_i(\mathbf{x},t)+\eta_i(\mathbf{x},t)\,. \tag{1}$$

The collision operator $\Omega_i^{(\mathrm{BGK})}$ can be written as

$$\Omega_i^{(\mathrm{BGK})}(\mathbf{x},t)=-\frac{1}{\tau}\left[f_i(\mathbf{x},t)-f_i^{(\mathrm{eq})}(\mathbf{x},t)\right], \tag{2}$$

where $\tau$ is the relaxation time and the equilibrium populations $f_i^{(\mathrm{eq})}(\mathbf{x},t)$ are defined from a second-order approximation of the Maxwell-Boltzmann distribution function

$$f_i^{(\mathrm{eq})}(\mathbf{x},t)=w_i n\left[1+\frac{\xi_i^\alpha u_\alpha^{(\mathrm{eq})}}{c_s^2}+\frac{\left(\xi_i^\alpha u_\alpha^{(\mathrm{eq})}\right)^2}{2c_s^4}-\frac{u_\alpha^{(\mathrm{eq})}u_\alpha^{(\mathrm{eq})}}{2c_s^2}\right], \tag{3}$$

where $c_s^2=1/3$ is the squre of the sound speed related to the D3Q19 stencil used for the simulations. The equilibrium velocity $u^\alpha_{(\mathrm{eq})}$ is suitably defined to take into account the force term $F^\alpha$ as

$$u^\alpha_{(\mathrm{eq})}(\mathbf{x},t)=\frac{1}{n(\mathbf{x},t)}\sum_{i=0}^{N_p-1}\xi_i^\alpha f_i(\mathbf{x},t)+\frac{1}{2n(\mathbf{x},t)}F^\alpha(\mathbf{x},t), \tag{4}$$

which needs to be paired with the population forcing term [3]

$$F_i=\left(1-\frac{1}{2\tau}\right)w_i\left[\frac{1}{c_s^2}\xi_i^\alpha+\frac{1}{c_s^4}\left(\xi_i^\alpha\xi_i^\beta-c_s^2\delta^{\alpha\beta}\right)u_\beta^{(\mathrm{eq})}\right]F_\alpha, \tag{5}$$

allowing the model to consistently recover all relevant thermodynamic properties [1, 2, 4]. The density gradients implementing phase-separation are triggered by the Shan-Chen (SC) force term [5, 6]

$$F^\mu(\mathbf{x},t)=-Gc_s^2\psi(\mathbf{x},t)\sum_{a=1}^{18}w\left(|\mathbf{e}_a|^2\right)\psi(\mathbf{x}+\mathbf{e}_a,t)\,e_a^\mu, \tag{6}$$

with $w(1)=1/6$ and $w(2)=1/12$ and $\mathbf{e}_a=\xi_a$ for $a=1,\dots,18$. For multi-phase and multi-component systems the SC model features also a lattice pressure tensor (LPT) [4, 7–9] that for the three-dimensional model in use reads

$$P^{\mu\nu}(\mathbf{x},t)=n(\mathbf{x},t)c_s^2\delta^{\mu\nu}+\frac{Gc_s^2}{2}\psi(\mathbf{x},t)\sum_{a=1}^{18}W\left(|\mathbf{e}_a|^2\right)\psi(\mathbf{x}+\mathbf{e}_a,t)\,e_a^\mu e_a^\nu. \tag{7}$$

Finally, the random variables $\{\eta_i\}$ are obtained as linear combinations of Gaussian random variables implicitly defined in moment space as $N_a=\sum_i m_{ai}\eta_i$, i.e. $\eta_i=\sum_a(m^{-1})_{ia}N_a$. The details for $m_{ai}$ are provided in Sec. III.

The link with the notation used in the main text is the following: (i) redefine the coupling constant as $-Gc_s^2\to G>0$, (ii) substitute the ideal term as $nc_s^2\to n$, then (iii) normalize the pressure by $G=T^{-1}$ in order to get Eq. (6) from the main text.

## II. HYDRODYNAMIC FLUCTUATIONS & MULTIPHASE SC-LBM STRUCTURE FUNCTION

### A. General Formulation

In this section we provide some details about the frameork of fluctuating hydrodynamics. More details can be found in [10, 11]. The variance for the random stress tensor $R^{\alpha\beta}$ is given in terms of the hydrodynamic fluctuations energy $k_B\vartheta$ by

$$\begin{aligned}&\langle R^{\alpha\beta}(\mathbf{x},t)R^{\mu\nu}(\mathbf{x}',t')\rangle\\&=2n_0k_B\vartheta\left[\nu_s\left(\delta^{\alpha\mu}\delta^{\beta\nu}+\delta^{\alpha\nu}\delta^{\beta\mu}\right)+\left(\nu_b-\frac{2}{d}\nu_s\right)\delta^{\alpha\beta}\delta^{\mu\nu}\right]\\&\quad\times\delta^{(3)}\left(\mathbf{x}-\mathbf{x}'\right)\delta\left(t-t'\right)\end{aligned} \tag{8}$$

where $\nu_s$ and $\nu_b$ are the shear and bulk kinematic viscosities, respectively [12, 13]. In the present case of single relaxation time LBM, Eq. (8) further simplifies given that the two viscosities are related by $\nu_b=2\nu_s/d$. The Fourier transform of the linearized Navier-Stokes equations for $\mathbf{u}(\mathbf{x},t)=\delta\mathbf{u}(\mathbf{x},t)$ and $n(\mathbf{x},t)=n_0+\delta n(\mathbf{x},t)$, read

$$\partial_t\delta\hat{n}-\imath n_0k_\alpha\delta\hat{u}^\alpha=0, \tag{9}$$

* shanxw@sustech.edu.cn

$$\partial_t \delta\hat{u}^{\alpha} = \frac{\imath k_{\beta}}{n_0}\left(\delta\hat{P}^{\alpha\beta} - \hat{R}^{\alpha\beta}\right) - \nu_{\mathrm{s}}\left(k^{\alpha}k_{\beta}\delta\hat{u}^{\beta} + |\mathbf{k}|^2\delta\hat{u}^{\alpha}\right) - \left(\nu_{\mathrm{b}} - \frac{2}{d}\nu_{\mathrm{s}}\right)k^{\alpha}k_{\gamma}\delta\hat{u}^{\gamma}. \tag{10}$$

The normalized wave-vector $\hat{k}^{\alpha} = k^{\alpha}/|\mathbf{k}|$ can be used to project vectors and tensors along the direction *parallel* to $\hat{k}^{\alpha}$ (indicated by the $||$ subscript) and the *orthogonal* one (indicated by $\perp$). For a generic vector $A^{\mu}$ or rank-two symmetric tensor $T^{\alpha\beta}$ one can leverage the projector along the orthogonal direction to $\hat{k}^{\alpha}$, i.e. $q^{\alpha\beta} = \delta^{\alpha\beta} - \hat{k}^{\alpha}\hat{k}^{\beta}$, and write

$$A_{||} = A_{\mu}\hat{k}^{\mu}, \quad A_{\perp}^{\mu} = A_{\alpha}q^{\alpha\mu}, \qquad T_{||} = \hat{k}_{\alpha}\hat{k}_{\beta}T^{\alpha\beta}, \quad T_{\perp}^{\alpha} = T^{\beta\gamma}\hat{k}_{\beta}q_{\gamma}^{\alpha}. \tag{11}$$

We notice that the continuity equation Eq. (9) is already projected onto the longitudinal velocity while for Eq. (10) the same projection reads

$$\partial_t \delta\hat{u}_{||} = \frac{\imath k}{n_0}\left(\delta\hat{P}_{||} - \hat{R}_{||}\right) - \nu_{||}k^2\delta\hat{u}_{||} \tag{12}$$

with $\nu_{||} = \nu_{\mathrm{b}} + 2(1-1/d)\,\nu_{\mathrm{s}}$. Now, we focus on the longitudinal projection of the variation of the Fourier-transformed pressure tensor $\delta\hat{P}$. We define the scale-dependent speed of sound $\bar{c}_s^2$ through the relation $\delta\hat{P}_{||} = \delta\hat{P}^{\mu\nu}\hat{k}_{\mu}\hat{k}_{\nu} = \bar{c}_s^2(k)\,\delta\hat{n}$. One can make use of Eq. (9) and solve for the longitudinal velocity as $\delta\hat{u}_{||} = -\imath\partial_t\delta\hat{n}/n_0 k$, which can be plugged into Eq. (12), thus yielding a second-order equation in time for $\delta\hat{n}$

$$\left[\partial_t^2 + \nu_{||}k^2\partial_t + k^2\bar{c}_s^2(k)\right]\delta\hat{n}(k,t) = -k^2\hat{R}_{||}, \tag{13}$$

which, after a Fourier transform in the time domain, can be used to express $\delta\hat{n}(\omega,k)$ as

$$\delta\hat{n}(k,\omega) = \frac{k^2\hat{R}_{||}(k,\omega)}{\omega^2 - k^2\bar{c}_s^2(k) + \imath\nu_{||}k^2\omega}. \tag{14}$$

thus yielding the dynamic structure factor as $S(\mathbf{k},\omega) = \langle|\delta\hat{n}(\mathbf{k},\omega)|^2\rangle$. Considering that $\langle|R_{||}(k,t)|^2\rangle = 2n_0k_B\vartheta\nu_{||}$, one can perform a contour integration over complex values of $\omega$ and obtain the general expression for the static structure factor

$$S(k) = \frac{n_0k_B\vartheta}{\bar{c}_s^2(k)}. \tag{15}$$

The specific expression of $\bar{c}_s^2(k)$ depends on the underlying model used for phase separation.

### B. Multi-Phase Shan-Chen Model

We begin by rewriting the lattice pressure tensor [4, 7, 14]

$$P^{\mu\nu}(\mathbf{x},t) = n(\mathbf{x},t)\,T\delta^{\mu\nu} - \frac{1}{2}\psi(\mathbf{x},t)\sum_{i=0}^{18}W\left(|\xi_i|^2\right)\psi(\mathbf{x}+\xi_i,t)\,\xi_i^{\mu}\xi_i^{\nu}. \tag{16}$$

When taking the spatial Fourier transform, the unit vector $\hat{k}^{\mu}$ lies along the direction of the density gradient $\partial^{\mu}\delta n$, so that when we consider the variation of the longitudinal projection of the pressure tensor, i.e. $\delta\hat{P}_{||} = \delta\hat{P}^{\mu\nu}\hat{k}_{\mu}\hat{k}_{\nu}$, one is actually selecting the normal component of the pressure tensor $P_{\mathrm{N}}$ with respect to the gradient of the local density fluctuations. Without loss of generality, one can assume $\hat{k} = \hat{x}$, so that $P_{\mathrm{N}} = P^{xx}$ which from Eq. (16) follows as

$$P_{\mathrm{N}}(x) = n(x)\,T\delta^{\mu\nu} - \frac{1}{4}\psi(x)\left[\psi(x+1) + \psi(x-1)\right]. \tag{17}$$

The expression above enjoys the fundamental property of yielding a constant value, up to machine precision, when evaluated across a flat interface [4, 14], i.e. $P_{\mathrm{N}} = P_0$. This represents an exact implementation on the discrete lattice of the *mechanic equilibrium* condition [15], i.e. any normal pressure gradient, even through the interface, would cause the latter to move. We can equivalently express Eq. (17) in terms of its Taylor expansion as

$$P_{\mathrm{N}}(x) = \left[n(x)\,T - \frac{1}{2}\psi^2(x)\right] - \frac{1}{2}\psi(x)\sum_{n=1}^{+\infty}\frac{1}{(2n)!}\frac{\mathrm{d}^{2n}}{\mathrm{d}x^{2n}}\psi(x),$$

of which we can take the variation with resepct to the density fluctuations as

$$\delta P_{\mathrm{N}}(x) = \left[T - \psi_0\psi_0'\right]\delta n(x) - \frac{1}{2}\psi_0\psi_0'\sum_{n=1}^{+\infty}\frac{1}{(2n)!}\frac{\mathrm{d}^{2n}}{\mathrm{d}x^{2n}}\delta n(x).$$

Finally, by taking the Fourier transform of the equation, and defining $\bar{c}_{s,0}^2 = T - \psi_0\psi_0'$, we obtain

$$\delta\hat{P}_{\mathrm{N}}(k) = \left\{\bar{c}_{s,0}^2 - \frac{1}{2}\psi_0\psi_0'\sum_{n=1}^{+\infty}\frac{(-)^n}{(2n)!}k^{2n}\right\}\delta\hat{n}(k), \tag{18}$$

and notice that the series can be summed finally yielding the exact expression

$$\bar{c}_s^2(k) = \bar{c}_{s,0}^2 - \frac{1}{2}\psi_0\psi_0'\left[\cos(k) - 1\right], \tag{19}$$

from which one can compute the sought-of expression for the static structure factor

$$S(k) = n_0k_B\vartheta\Big/\left\{\bar{c}_{s,0}^2 - \frac{1}{2}\psi_0\psi_0'\left[\cos(k) - 1\right]\right\}. \tag{20}$$

In [10] a free-energy model was adopted and the results were later extended to the Shan-Chen model in [11] where $\bar{c}_s^2(k)$ was approximated up to $O(k^2)$. A mismatch ($\gtrsim 15\%$) between the numecial values of the structure factor $S(k)$ and its theoretical expression were reported in [11]. The latter may be due to (i) the low approximation order and (ii) the use of an approximate expression for the pressure tensor derived from the Taylor expansion of the force in Eq. (6) rather than the lattice version Eq. (7).

As discussed in the main text, it is possible to rearrange the terms and obtain a direct mapping onto the functional form

of the momentum-space propagator of the Gaussian Ising model [16]

$$G_0(k) = \frac{S(k)}{n_0 k_B \vartheta}\left(c_s^2 + \frac{1}{2}\psi_0\psi_0'\right) = \frac{1}{1-2\beta\cos(k)}, \quad (21)$$

with the inverse temperature defined as

$$2\beta = \frac{\psi_0\psi_0'/2}{T+\psi_0\psi_0'/2} = \frac{1}{1+2/(\psi_0\psi_0')} > 0. \quad (22)$$

## III. LBM SIMULATIONS

### A. Populations noise variance

As detailed in [11] one only needs to specify the variance of the noise moments $N_a = \sum_i m_{ai}\eta_i$, where $\eta_i$ is the population noise appearing in the stochastic LB equation (2). In order to guarantee exact conservation of density and momentum, one needs to set the variance of the related stochastic moments to zero, i.e. ordering the moments as reported in Table I one can write a diagonal covariance matrix as follows

$$\Xi_{ab} = \langle N_a N_b \rangle = \frac{n_0 k_B \vartheta}{c_s^2}\frac{1}{\tau}\left(2-\frac{1}{\tau}\right)\mathrm{diag}\left[0,0,0,0,M_4,\ldots,M_{18}\right], \quad (23)$$

where $M_a = \sum_i w_i m_{ai}^2$ represent the *norm* of the moments over the weighted scalar product in the population space. Eq. (23) implies that all the stochastic moments are simply uncorrelated Gaussian random numbers that can be independently computed via Box-Müller transform [17] starting from two uniformly distributed pseudo-random numbers. The most important property of the moments $m_{ai}$ is their orthogonality with respect to the weighted scalar product in population space, i.e. $\delta_{ab} = \sum_i w_i m_{ai} m_{bi}$. While for the two-dimensional case it is enough to consider a basis given by Hermite polynomials, in three dimensions this is no longer possible because of the non-hydrodynamic higher-order ghost moments [1, 2]. Hence, we resorted to the Gram-Schmidt orthogonalization over some set of three-dimensional Hermite polynomial yielding the results reported in Table I.

### B. Data Analysis

The discrete Fourier transform are performed in a straightforward way as described in the definition of the Fourier transform for the spin-glass susceptibility in [18]. Given that $S(k)$ only depends on the norm of $\mathbf{k}$ and that it is given by the complex norm of $\delta n(k)$ then one can average the results obtained along the three directions

$$\mathbf{k}_x = (k,0,0), \quad \mathbf{k}_y = (0,k,0), \quad \mathbf{k}_z = (0,0,k), \quad (24)$$

and simply compute the squared norm as

$$|\delta\hat{n}_x(k,t)|^2 = \frac{1}{L}\sum_x \left\{\left[\delta n_{yz}(x)\cos(kx)\right]^2 + \left[\delta n_{yz}(x)\sin(kx)\right]^2\right\}, \quad (25)$$

where we defined the plane average as

$$\delta n_{yz}(x) = \frac{1}{L^2}\sum_{y,z}\delta n(x,y,z). \quad (26)$$

One can repeat the computation for the three different direction for a sequence of time values $t = 1,\ldots,T$ and obtain the steady-state average as

$$\langle|\delta\hat{n}(k)|^2\rangle = \frac{1}{T}\sum_{t=1}^{T}\frac{1}{3}\left[|\delta n_x(k,t)|^2 + |\delta n_y(k,t)|^2 + |\delta n_z(k,t)|^2\right]. \quad (27)$$

The values for $\cos(kx)$ and $\sin(kx)$ can be stored in look-up tables for each value of $k = 2\pi n_k/L$ with $n_k = 1,\ldots,\lfloor L/2\rfloor$, thus computing them only once.


[1] T. Krüger, H. Kusumaatmaja, A. Kuzmin, O. Shardt, G. Silva, and E. M. Viggen, *The lattice Boltzmann method* (Springer, 2017).

[2] S. Succi, *The lattice Boltzmann equation: for complex states of flowing matter* (Oxford University Press, 2018).

[3] Z. Guo, C. Zheng, and B. Shi, Discrete lattice effects on the forcing term in the lattice Boltzmann method, Physical Review E **65**, 046308 (2002).

[4] M. Lulli, L. Biferale, G. Falcucci, M. Sbragaglia, and X. Shan, Structure and isotropy of lattice pressure tensors for multirange potentials, Physical Review E **103**, 10.1103/physreve.103.063309 (2021).

[5] X. Shan and H. Chen, Lattice Boltzmann model for simulating flows with multiple phases and components, Physical Review E **47**, 1815 (1993).

[6] X. Shan and H. Chen, Simulation of nonideal gases and liquid-gas phase transitions by the lattice Boltzmann equation, Physical Review E **49**, 2941 (1994).

[7] X. Shan, Pressure tensor calculation in a class of nonideal gas lattice Boltzmann models, Physical Review E **77**, 066702 (2008).

[8] M. Sbragaglia and D. Belardinelli, Interaction pressure tensor for a class of multicomponent lattice Boltzmann models, Physical Review E **88**, 013306 (2013), arXiv:1305.2547.

[9] C. S. From, E. Sauret, S. A. Galindo-Torres, and Y. T. Gu, Interaction pressure tensor on high-order lattice Boltzmann models for nonideal fluids, Physical Review E **99**, 063318 (2019).

[10] M. Gross, R. Adhikari, M. E. Cates, and F. Varnik, Thermal fluctuations in the lattice boltzmann method for nonideal fluids, Physical Review E **82**, 10.1103/physreve.82.056714 (2010).

[11] M. Gross, R. Adhikari, M. E. Cates, and F. Varnik, Modelling thermal fluctuations in non-ideal fluids with the lattice boltzmann method, Philosophical Transactions of the Royal Society A: Mathematical, Physical and Engineering Sciences **369**, 2274

| $(a,i)$ | $m_{ai}$ | $M_a$ | $w_i$ | $\boldsymbol{\xi}_i$ |
|---|---|---|---|---|
| 0 | $1$ | $1$ | $1/3$ | $(0,0,0)$ |
| 1 | $\xi_i^x$ | $1/3$ | $1/18$ | $(1,0,0)$ |
| 2 | $\xi_i^y$ | $1/3$ | $1/18$ | $(0,1,0)$ |
| 3 | $\xi_i^z$ | $1/3$ | $1/18$ | $(-1,0,0)$ |
| 4 | $\left(\xi_i^x\right)^2-\frac{1}{3}$ | $2/9$ | $1/18$ | $(0,-1,0)$ |
| 5 | $\xi_i^x\xi_i^y$ | $1/9$ | $1/18$ | $(0,0,1)$ |
| 6 | $\xi_i^x\xi_i^z$ | $1/9$ | $1/18$ | $(0,0,-1)$ |
| 7 | $\left(\xi_i^y\right)^2-\frac{1}{3}$ | $2/9$ | $1/36$ | $(1,1,0)$ |
| 8 | $\xi_i^y\xi_i^z$ | $1/9$ | $1/36$ | $(-1,1,0)$ |
| 9 | $\left(\xi_i^z\right)^2-\frac{1}{3}$ | $2/9$ | $1/36$ | $(-1,-1,0)$ |
| 10 | $\xi_i^y\left(\left(\xi_i^x\right)^2-\frac{1}{3}\right)$ | $2/27$ | $1/36$ | $(1,-1,0)$ |
| 11 | $\xi_i^z\left(\left(\xi_i^x\right)^2-\frac{1}{3}\right)$ | $2/27$ | $1/36$ | $(1,0,1)$ |
| 12 | $\xi_i^x\left(\left(\xi_i^y\right)^2-\frac{1}{3}\right)$ | $2/27$ | $1/36$ | $(-1,0,1)$ |
| 13 | $\frac{1}{2}\xi_i^x\left(\left(\xi_i^y\right)^2+2\left(\xi_i^z\right)^2-1\right)$ | $1/18$ | $1/36$ | $(-1,0,-1)$ |
| 14 | $\frac{1}{2}\xi_i^z\left(\left(\xi_i^x\right)^2+2\left(\xi_i^y\right)^2-1\right)$ | $1/18$ | $1/36$ | $(1,0,-1)$ |
| 15 | $\frac{1}{2}\xi_i^y\left(\left(\xi_i^x\right)^2+2\left(\xi_i^z\right)^2-1\right)$ | $1/18$ | $1/36$ | $(0,1,1)$ |
| 16 | $\left(\xi_i^x\right)^2\left(\xi_i^y\right)^2-\frac{1}{3}\left(\xi_i^x\right)^2-\frac{1}{3}\left(\xi_i^y\right)^2+\frac{1}{6}\left(\xi_i^z\right)^2+\frac{1}{18}$ | $7/162$ | $1/36$ | $(0,-1,1)$ |
| 17 | $\frac{2}{7}\left(\xi_i^x\right)^2\left(\xi_i^y\right)^2+\left(\xi_i^x\right)^2\left(\xi_i^z\right)^2-\frac{3}{7}\left(\xi_i^x\right)^2+\frac{1}{14}\left(\xi_i^y\right)^2-\frac{2}{7}\left(\xi_i^z\right)^2+\frac{1}{14}$ | $5/126$ | $1/36$ | $(0,-1,-1)$ |
| 18 | $\frac{2}{5}\left(\xi_i^x\right)^2\left(\xi_i^y\right)^2+\frac{2}{5}\left(\xi_i^x\right)^2\left(\xi_i^z\right)^2-\frac{1}{10}\left(\xi_i^x\right)^2+\left(\xi_i^y\right)^2\left(\xi_i^z\right)^2-\frac{2}{5}\left(\xi_i^y\right)^2-\frac{2}{5}\left(\xi_i^z\right)^2+\frac{1}{10}$ | $1/30$ | $1/36$ | $(0,1,-1)$ |

Table I. Table

(2011).

[12] L. LANDAU, E. LIFSHITZ, and R. Beyer, Hydrodynamic fluctuations, in *Perspectives in Theoretical Physics* (Elsevier, 1992) pp. 359–361.

[13] L. P. Pitaevskii and E. M. Lifshitz, *Statistical Physics, Part 2: Volume 9 (Course of Theoretical Physics Vol. 9)* (Butterworth-Heinemann, 1980).

[14] M. Sbragaglia, R. Benzi, L. Biferale, S. Succi, K. Sugiyama, and F. Toschi, Generalized lattice Boltzmann method with multirange pseudopotential, Physical Review E **75**, 026702 (2007).

[15] J. S. Rowlinson, The critical exponent of Tolman's length, Journal of Physics A: Mathematical and General **17**, L357 (1984).

[16] G. Parisi, *Statistical Field Theory* (Avalon Publishing, 1998).

[17] G. E. P. Box and M. E. Muller, A note on the generation of random normal deviates, The Annals of Mathematical Statistics **29**, 610 (1958).

[18] M. Lulli, G. Parisi, and A. Pelissetto, Out-of-equilibrium finite-size method for critical behavior analyses, Physical Review E **93**, 10.1103/physreve.93.032126 (2016).
